# Supplementary material for: Prompt-Augmented Linear Probing: Scaling beyond the Limit of Few-shot In-Context Learners
Source: arXiv:2212.10873 source file (2023-06-14)
Supplement: Supplementary file 1 [file 99.Appendix.tex]

\clearpage
\appendix

    \section{Method Description \& Implementation Details}
        This section describes the specific implementation and hyper-parameters of each model used in the experiment.

    \begin{itemize}
        \item \textbf{$k$-Nearest Neighbors ($k$-NN)}:  the $k$-NN is a non-parametric supervised learning method that outputs a class membership by assigning the most common class label among its $k$ nearest neighbors. Specifically, we set $k$ to 3 and leverage euclidean distance to select the nearest samples. 
        
        % $k$ =3 and euclidean distance 
        \item \textbf{Support Vector Machine (SVM)}: The goal of SVM is to find the hyperplane that separates the group of data points $x_{i}$ with \textit{maximum-margin}:
        \[ w^{T}h-b = 0,\]
        \noindent where $w$ is the normal vector to the hyperplane.
        We trained SVM with the linear kernel (linear) and used squared hinge loss.
        
        \item \textbf{Logistic Regression (LR)}: LR is a statistical model that models the probability of each class by having the combination of log odds from independent features:
        \[p(y|h)= Ber(y|\sigma(w^{T}h+b)),\]
        where $\sigma$ is the sigmoid activation, $w$ and $b$ refers to weights and bias.
        Then the probability of input $h$ belonging to class $y=1$ can be written as follows:
        \[p(y=1|h)= \sigma(a),\]
        where $Ber$ is bernoulli distribution, $a = w^{T}h+b$ usually termed as \textit{logit} which is combination of log odds from variables.
        \item \textbf{Single layer perceptron (SLP)}: SLP is a single-layer version of the neural network, which we commonly use in machine learning literature:
            \[p(y|x) = softmax(w\sigma(h) + b),\]
        \noindent where $\sigma$ refers to an activation function.
        To train SLP, we used ReLU activation, cross-entropy loss, and Adam optimizer with a learning rate of 15e-5. For the training batch size, we set it to 2 for the few-shot setting and 16 for the full-training dataset.

        \item \textbf{Gaussian discriminative analysis (GDA)} :
        GDA is a generative classification method, unlike other probing methods mentioned above.
        Generative classifiers classify the given input via the Bayes rule, while discriminative classifier directly models the class posterior:
            \begin{equation}
                p(y=c|\bm{h;\theta}) = \frac{p(\bm{h}|y=c;\bm{\theta}) p(y=c;\bm{\theta})}{\Sigma_{c^{*}\in|C|}p(\bm{h}|y=c^{*};\bm{\theta}) p(y=c^{*};\bm{\theta})}.
            \end{equation}
        Formally, they estimate posterior from the class likelihood $p(\bm{h}|y=c;\bm{\theta})$ and prior distribution $p(y=c;\bm{\theta})$.
        Then GDA computes the most probable class label as follows :
        
        \begin{equation}
        \begin{aligned}
        \hat{y}(h)&=\argmax_{i^*} \text{log}p(y=i^*|h). \\ 
        &= \argmin_{i^*}(h=\mu_c)^T\Sigma^{-1}(h-\mu_c)
        \end{aligned}    
        \end{equation}
        
        Meaning GDA classifies new input with the label $i^*$ which has closest Mahalanobis distance (i.e., $(h=\mu_c)^T\Sigma^{-1}(h-\mu_c)$).
        We estimate tied (shared) covariance $\Sigma$ of GDA with the Ledoit-wolf shrinkage method \cite{ledoit2004honey}.
        
        \item \textbf{In-Context Learning (ICL)}: In-context learning (ICL) is a training-free paradigm that attempts to generate the desired output by guiding the model with a few examples of the target task (i.e., demonstrations) plus a set of templates tailored for the task. 
        Formal descriptions are in the main paper.
        The template and verbalizer for each task are in Table \ref{tab:templates}.
        Specifically, if only input comes as an input $f_{\text{template}}(x_i)$ the label is left blank, and when a label also comes as a pair $f_{\text{template}}(x_i,y_i)$, a verbalizer transforms label into a natural language label.
        
        Verbalizer for some tasks (i.e., CLINC, BANKING, BoolQ, CB) is not defined as not viable through ICL since they are too long (BoolQ, CB) or has too many classes (CLINC, BANKING).
        These tasks are used in the PALP-T method that applies only templates without attaching demonstrations.
        
        % single token natural language label -> details in table
        \item \textbf{Fine-tuning \& Adapter}: 
        Fine-tuning and Adapter are representative \textit{white-box tuning} methodologies.
        The training process is analogous to SLP, which utilizes cross-entropy loss with gradient descent.
        
        For fine-tuning, we used AdamW \cite{loshchilov2017decoupled} optimizer with epsilon 1e-5, weight decay 0.1 and set the batch size to 8.
        Additionally, we used deepspeed \cite{rajbhandari2020zero} to train models.
        Specifically, we used ZeRO2 with CPU offload on a 240GB RAM CPU.
        In this setting, fine-tuning GPT-J on CLINC150 full dataset takes about 7.1 GPU hours per epoch. 
        
        For the adapter, we utilize the baseline adapter proposed in \citet{houlsby2019parameter} with additional 1\% of the backbone PLM.
        We used AdamW \cite{loshchilov2017decoupled} optimizer with epsilon 1e-5, weight decay 0.1 and set the batch size to 8.

    \end{itemize}

 \section{Datasets in Details}
        We utilized 15 different datasets ranging from binary tasks to multi-class classification tasks in single sentence tasks and sentence pair tasks in various domains as follows: SST2, CoLA, MRPC, RTE, and MNLI datasets from GLUE benchmark \cite{wang2018glue}, BoolQ, and 
        CB datasets from SuperGLUE \cite{wang2019superglue}, stance\_atheism, and emotion datasets from tweet eval \cite{barbieri2020tweeteval}, and AGnews \cite{Zhang2015CharacterlevelCN}, Rotten tomatoes \cite{Pang+Lee:05a}, TREC \cite{li-roth-2002-learning}, CLINC \cite{larson2019evaluation}, and Banking77 \cite{casanueva-etal-2020-efficient} datasets.

    \section{Additional Experimental Results}
        This section reports performance results on additional shots (8-shot, 16-shot) and standard deviation for each methodology.
        If the task cannot be solved due to length limitation, it is marked within the Table.
        
\begin{table*}[t]
\centering
\begin{tabular}{@{}c|l|l@{}}
\toprule
\multicolumn{1}{c|}{Task type}  & \multicolumn{1}{c|}{Dataset} & \multicolumn{1}{c}{Template} \\
\midrule
\multirow{10}{*}{Single} & SST2 & Sentence 1: [sent1]$\backslash$nSentiment: [positive / negative] \\
 & Rotten\_Tomatoes & Sentence 1: [sent1]$\backslash$nSentiment: [positive / negative] \\
 & Offensive & Sentence 1: [sent1]$\backslash$nSentiment: [non-offensive / offensive] \\
 & CoLA & Sentence 1: [sent1]$\backslash$nSentiment: [correct / wrong] \\
 & Stance\_atheism & Sentence 1: [sent1] Label: [none / against / favor] \\
 & Emotion & Sentence 1: [sent1]$\backslash$nSentiment: [anger / joy / optimism / sadness] \\
 & AGnews & Sentence 1: [sent1]$\backslash$nSentiment: [World / Sports / Business / Technology] \\
 & TREC & Sentence 1: [sent1]$\backslash$nLabel: [Description / Entity / Expression / Human / Number / Location] \\
 & Banking 77 & Sentence 1: [sent1] Label: [] \\
 & CLINC 150 & Sentence 1: [sent1]$\backslash$nLabel: [] \\
 \midrule
\multirow{6}{*}{Pair} & mnli & Sentence 1: [sent1]$\backslash$nSentence 2: [sent2]$\backslash$nLabel: [True / Neither / False] \\
 & MRPC & Sentence 1: [sent1]$\backslash$nSentence 2: [sent2]$\backslash$nLabel: [True / False] \\
 & RTE & Premise: [sent1]$\backslash$nHypothesis: [sent2]$\backslash$nLabel: [True / False] \\
 & BoolQ & Premise: [sent1]$\backslash$nHypothesis: [sent2]$\backslash$nLabel: [] \\
 & CB & Premise: [sent1]$\backslash$nHypothesis: [sent2]$\backslash$nLabel: [] \\
%  & qnli & Premise: [sent1]$\backslash$nHypothesis: [sent2]$\backslash$nLabel: [positive, negative]\\
 \bottomrule
\end{tabular}
\caption{A list of template and verbalizer for each dataset.}
\label{tab:templates}
\end{table*}

\settowidth\rotheadsize{Minimal}
\begin{table*}[t]
\centering
\resizebox{2 \columnwidth}{!}{

    \begin{tabular}{c|c|cccccccccccc} 
    \hline
    \multicolumn{14}{c}{GPT-J 4-shot per class}                                                                                                                         \\ 
    \hline
    \multicolumn{2}{c|}{Method}                 & AG    & SST-2 & RT    & Stance & Emotion & TREC  & CoLA  & Offensive & MNLI  & RTE   & MRPC  & AVG                     \\ 
    \hline
    \multirow{10}{*}{B} & \multirow{2}{*}{k-NN} & 54.66 & 51.33 & 58.67 & 54.73  & 33.92   & 48.84 & 42.36 & 49.37     & 35.09 & 48.74 & 64.66 & \multirow{2}{*}{49.31}  \\
                        &                       & $\pm$7.5   & $\pm$3.5   & $\pm$6.9   & $\pm$9.8    & $\pm$2.6     & $\pm$7     & $\pm$8.3   & $\pm$13.9      & $\pm$1.4   & $\pm$2.9   & $\pm$1.2   &                         \\
                        & \multirow{2}{*}{LR}   & 66.48 & 50.25 & 65.08 & 58.64  & 36.89   & 64.48 & 50.68 & 51.72     & 36.46 & 49.39 & 59.02 & \multirow{2}{*}{53.55}  \\
                        &                       & $\pm$2.7   & $\pm$1.1   & $\pm$8.4   & $\pm$4.2    & $\pm$2.6     & $\pm$7.9   & $\pm$10.6  & $\pm$9.5       & $\pm$1.9   & $\pm$3.9   & $\pm$3.9   &                         \\
                        & \multirow{2}{*}{SVM}  & 66.20  & 50.41 & 65.91 & 59.27  & 36.59   & 65.92 & 48.90  & 48.72     & 36.02 & 49.31 & 61.96 & \multirow{2}{*}{53.56}   \\
                        &                       & $\pm$2.5   & $\pm$1.2   & $\pm$8.6   & $\pm$4.3    & $\pm$2.4     & $\pm$5.9   & $\pm$9.6   & $\pm$7         & $\pm$1.7   & $\pm$4.2   & $\pm$2.5   &                         \\
                        & \multirow{2}{*}{SLP}   & 67.88 & 50.23 & 65.68 & 59.45  & 37.13   & 66.80  & 49.13 & 49.95     & 36.36 & 49.24 & 61.76 & \multirow{2}{*}{53.96}  \\
                        &                       & $\pm$3.1   & $\pm$1.4   & $\pm$9     & $\pm$2.9    & $\pm$3.9     & $\pm$6     & $\pm$9.9   & $\pm$5.9       & $\pm$2     & $\pm$3.8   & $\pm$2.2   &                         \\
                        & \multirow{2}{*}{GDA}  & 66.32 & 50.41 & 65.93 & 58.64  & 36.88   & 66.44 & 48.88 & 48.72     & 36.03 & 49.24 & 61.96 & \multirow{2}{*}{53.59}  \\
                        &                       & $\pm$2.9   & $\pm$1.2   & $\pm$8.6   & $\pm$4.1    & $\pm$2.4     & $\pm$7     & $\pm$9.6   & $\pm$7         & $\pm$1.8   &$\pm$4.3   &$\pm$2.5   &                         \\ 
    \hline
    \multirow{10}{*}{T} & \multirow{2}{*}{k-NN} & 61.88 & 58.30  & 65.10  & 35.27  & 45.18   & 51.04 & 53.02 & 59.98     & 36.40  & 53.14 & 61.47 & \multirow{2}{*}{52.80}  \\
                        &                       &$\pm$4.1   &$\pm$8.0    &$\pm$8.2   & $\pm$8.6    & $\pm$2.6     & $\pm$8.5   &$\pm$6.9   & $\pm$6         & $\pm$1.9   & $\pm$3.9   & $\pm$11.3  &                         \\
                        & \multirow{2}{*}{LR}   & 71.84 & 62.00    & 71.73 & 58.09  & 50.56   & 65.56 & 49.86 & 59.00        & 38.73 & 50.54 & 60.44 & \multirow{2}{*}{58.03}  \\
                        &                       & $\pm$2.2   & $\pm$9.6   &$\pm$8.6   & $\pm$7.2    & $\pm$5.8     & $\pm$6.54  &$\pm$1.6   &$\pm$9.8       &$\pm$3.4   &$\pm$3.5   &$\pm$7.4   &                         \\
                        & \multirow{2}{*}{SVM}  & 72.08 & 63.67 & 71.33 & 56.27  & 50.27   & 66.36 & 53.08 & 62.02     & 37.93 & 49.60  & 61.18 & \multirow{2}{*}{58.53}  \\
                        &                       &$\pm$2.1   & $\pm$8     & $\pm$9     &$\pm$7.8    &$\pm$4.2     &$\pm$8.9   &$\pm$2.4   &$\pm$10.1      &$\pm$3.3   &$\pm$3.9   &$\pm$8.2   &                         \\
                        & \multirow{2}{*}{SLP}   & 73.79 & 63.58 & 72.18 & 57.45  & 52.71   & 68.44 & 53.81 & 63.07     & 38.25 & 49.96 & 61.57 & \multirow{2}{*}{59.53}   \\
                        &                       &$\pm$2.6   &$\pm$8.5   &$\pm$9.3   &$\pm$6.8    &$\pm$5.9     &$\pm$7.5   &$\pm$1.6   &$\pm$7.4       &$\pm$3.4   &$\pm$3.3   &$\pm$7.1   &                         \\
                        & \multirow{2}{*}{GDA}  & 72.82 & 64.20  & 71.33 & 56.27  & 52.86   & 66.00    & 53.08 & 62.02     & 38.13 & 49.60  & 61.18 & \multirow{2}{*}{58.86}  \\
                        &                       &$\pm$2.2   &$\pm$7.5   & $\pm$9     &$\pm$7.8    &$\pm$5.2     &$\pm$9.2   &$\pm$2.4   &$\pm$10.1      &$\pm$3.4   &$\pm$3.9   &$\pm$8.2   &                         \\ 
    \hline 
    \multirow{10}{*}{D} & \multirow{2}{*}{k-NN} & 75.99 & 70.16 & 71.01 & 49.45  & 56.95   & 46.80 & 55.67 & 54.56     & 38.85 & 51.09 & 63.86 & \multirow{2}{*}{57.67}  \\
                        &                       &$\pm$5.6   &$\pm$7.7   &$\pm$12.3  &$\pm$12.9   & $\pm$6.0       &$\pm$6.3   &$\pm$10.9  & $\pm$6.0         &$\pm$2.2   &$\pm$5.1   &$\pm$9.4   &                         \\
                        & \multirow{2}{*}{LR}   & 77.92 & 70.62 & 80.58  & 61.27  & 68.97   & 65.96 & 53.83 & 67.63      & \textbf{40.30}  & 49.00    & 62.27 & \multirow{2}{*}{63.49}  \\
                        &                       &$\pm$4.6   &$\pm$12.2  &$\pm$6.2   &$\pm$11.0     &$\pm$4.3     &$\pm$6.9   &$\pm$8.5   &$\pm$6.9       & $\pm$4.0     &$\pm$3.3   &$\pm$9.5   &                         \\
                        & \multirow{2}{*}{SVM}  & 77.96    & 75.46 & 79.42 & 55.82  & 68.91   & 66.24 & 55.30 & 63.75     & 40.12 & 51.54 & 64.76 & \multirow{2}{*}{63.57}  \\
                        &                       &$\pm$4.6   & $\pm$10.0    &$\pm$7.5   &$\pm$10.5   &$\pm$3.7     &$\pm$7.0    &$\pm$7.4   &$\pm$3.3       &$\pm$2.9   &$\pm$6.0    &$\pm$7.9   &                         \\
                        & \multirow{2}{*}{SLP}   & 80.69 & 77.41 & 81.01 & \textbf{71.36}  & 70.38   & \textbf{71.92} & \textbf{69.13} & 72.35     & 39.41 & 54.66 & \textbf{71.73} & \multirow{2}{*}{\textbf{69.1}}   \\
                        &                       &$\pm$4.5   &$\pm$11.5  &$\pm$7.6   &$\pm$6.8    &$\pm$3.6     &$\pm$6.1   &$\pm$9.6   &$\pm$10.8      &$\pm$2.9   &$\pm$2.7   &$\pm$2.6   &                         \\
                        & \multirow{2}{*}{GDA}  & 76.08 & 70.16 & 68.05 & 55.91  & 65.66    & 63.76 & 54.42 & 69.18     & 39.32 & 50.53 & 64.15 & \multirow{2}{*}{61.57}  \\
                        &                       &$\pm$5.3   &$\pm$8.6   &$\pm$8.2   &$\pm$14.5   &$\pm$5.0      &$\pm$5.8   &$\pm$5.2   &$\pm$3.6       &$\pm$2.4   &$\pm$5.0    &$\pm$6.8   &                         \\ 
    \hline
    \multicolumn{2}{c|}{\multirow{2}{*}{ICL}}   & \textbf{81.74} & \textbf{91.77} & \textbf{90.45} & 23.09  & \textbf{72.76}   & 64.00    & 37.89 & \textbf{73.19}     & 36.04 & \textbf{55.60}  & 68.38 & \multirow{2}{*}{63.17}  \\
    \multicolumn{2}{c|}{}                       &$\pm$2.0    &$\pm$0.8   &$\pm$0.6   &$\pm$13.8   &$\pm$7.4     &$\pm$4.6   &$\pm$14.2  &$\pm$1.0        &$\pm$0.4   &$\pm$1.4   &$\pm$0.2   &                         \\
    \hline
    \end{tabular}

}
\caption{Experimental results on GPT-J in 4-shot per class settings. B, T, and D refers to a baseline, template, and demonstration individually. - means the case where ICL could not leverage full samples due to the length limitation. For each dataset, the \textbf{best method} is in bold. }

\label{tab:appendix_few-shot_4}
\end{table*}

\settowidth\rotheadsize{Minimal}
\begin{table*}[t]
\centering
\resizebox{2 \columnwidth}{!}{

    \begin{tabular}{c|c|cccccccccccc} 
    \hline
    \multicolumn{14}{c}{GPT-J 8-shot per class}                                                                                                                         \\ 
    \hline
    \multicolumn{2}{c}{Method}                  & AG    & SST-2 & RT    & Stance & Emotion & TREC  & CoLA  & Offensive & MNLI  & RTE   & MRPC  & AVG                     \\ 
    \hline
    \multirow{10}{*}{B} & \multirow{2}{*}{k-NN} & 63.05 & 50.55 & 65.42 & 58.09  & 36.05   & 60.16 & 52.41 & 52.26     & 35.69 & 51.7  & 59.17 & \multirow{2}{*}{53.14}  \\
                        &                       &$\pm$3.4   &$\pm$2.0    &$\pm$5.2   &$\pm$8.4    &$\pm$1.1     &$\pm$5.6   &$\pm$7.5   & $\pm$17.0z        &$\pm$0.5   &$\pm$3.0    &$\pm$10.3  &                         \\
                        & \multirow{2}{*}{LR}   & 74.56 & 57.50  & 74.15 & 65.73  & 41.90    & 79.08 & 52.79 & 58.47     & 37.43 & 51.34 & 58.97 & \multirow{2}{*}{59.27}  \\
                        &                       &$\pm$1.7   &$\pm$4.5   &$\pm$5.2   &$\pm$3.5    &$\pm$2.7     &$\pm$3.5   &$\pm$5.0    &$\pm$6.5       &$\pm$1.0    &$\pm$2.6   &$\pm$3.9   &                         \\
                        & \multirow{2}{*}{SVM}  & 73.26 & 57.16 & 75.87 & 64.27  & 42.66   & 80.12 & 53.98 & 57.79     & 37.43 & 52.06 & 59.56 & \multirow{2}{*}{59.47}  \\
                        &                       &$\pm$2.4   &$\pm$4.8   &$\pm$4.8   &$\pm$2.1    &$\pm$2.6     &$\pm$2.9   &$\pm$4.0    &$\pm$7.4       &$\pm$0.8   &$\pm$2.3   &$\pm$2.7   &                         \\
                        & \multirow{2}{*}{SLP}   & 74.72 & 57.91 & 75.25 & 63.82  & 42.87   & 80.92 & 54.34 & 55.93     & 37.37 & 51.05 & 59.46 & \multirow{2}{*}{59.42}  \\
                        &                       &$\pm$2.4   &$\pm$4.6   &$\pm$5.1   &$\pm$3.2    &$\pm$3.5     &$\pm$2.4   &$\pm$3.7   &$\pm$6.6       &$\pm$0.9   &$\pm$2.1   &$\pm$2.8   &                         \\
                        & \multirow{2}{*}{GDA}  & 74.12 & 57.16 & 75.78 & 63.00     & 44.31   & \textbf{81.84} & 53.98 & 57.79     & 37.6  & 52.06 & 59.56 & \multirow{2}{*}{59.75}  \\
                        &                       &$\pm$2.5   &$\pm$4.8   &$\pm$4.8   &$\pm$2.0     &$\pm$3.1     &$\pm$2.1   &$\pm$4.0    &$\pm$7.4       &$\pm$0.8   &$\pm$2.3   &$\pm$2.7   &                         \\ 
    \hline
    \multirow{10}{*}{T} & \multirow{2}{*}{k-NN} & 69.65 & 61.93 & 65.46 & 56.45  & 49.87   & 62.44 & 45.29 & 56.35     & 38.13 & 50.90  & 56.42 & \multirow{2}{*}{55.72}  \\
                        &                       &$\pm$3.7   &$\pm$6.9   &$\pm$4.9   &$\pm$4.1    &$\pm$4.8     &$\pm$5.7   &$\pm$5.0    &$\pm$3.6       &$\pm$1.4   &$\pm$2.4   &$\pm$12.5  &                         \\
                        & \multirow{2}{*}{LR}   & 78.52 & 69.33 & 77.04 & 66.00     & 59.93   & 79.04 & 51.51 & 59.30      & 41.24 & 52.56 & 63.48 & \multirow{2}{*}{63.45}  \\
                        &                       &$\pm$1.5   &$\pm$7.2   &$\pm$5.0    &$\pm$4.3    &$\pm$7.4     &$\pm$5.4   &$\pm$3.3   &$\pm$8.3       &$\pm$1.9   &$\pm$3.0    &$\pm$6.2   &                         \\
                        & \multirow{2}{*}{SVM}  & 78.39 & 75.44 & 77.97 & 63.36  & 60.53   & 81.12 & 51.98 & 65.07     & 40.45 & 53.07 & 61.13 & \multirow{2}{*}{64.41}  \\
                        &                       &$\pm$1.8   &$\pm$9.1   &$\pm$5.6   &$\pm$4.4    &$\pm$6.7     &$\pm$4.0    &$\pm$2.6   &$\pm$8.9       &$\pm$1.9   &$\pm$3.2   &$\pm$6.5   &                         \\
                        & \multirow{2}{*}{SLP}   & 79.61 & 72.80  & 78.03 & 66.09  & 62.36   & 80.12 & 52.10  & 64.37     & 40.87 & 52.49 & 61.67 & \multirow{2}{*}{64.59}  \\
                        &                       &$\pm$1.7   &$\pm$8.6   &$\pm$5.4   &$\pm$3.8    &$\pm$6.8     &$\pm$4.6   &$\pm$2.6   &$\pm$7.8       &$\pm$1.9   &$\pm$2.8   &$\pm$6.2   &                         \\
                        & \multirow{2}{*}{GDA}  & 79.03 & 75.37 & 77.90  & 62.55  & 62.15   & 81.68 & 51.98 & 65.05     & 40.9  & 53.07 & 61.18 & \multirow{2}{*}{64.62}  \\
                        &                       &$\pm$2.2   &$\pm$9.3   &$\pm$5.6   &$\pm$4.0     &$\pm$6.3     &$\pm$3.5   &$\pm$2.6   &$\pm$9.2       &$\pm$2.2   &$\pm$3.2   &$\pm$6.5   &                         \\ 
    \hline
    \multirow{10}{*}{D} & \multirow{2}{*}{k-NN} & 79.21 & 67.98 & 78.82 & 49.63   & 58.31   & 58.36 & 50.43 & 63.26     & 38.24 & 51.37 & 56.94 & \multirow{2}{*}{59.32}  \\
                        &                       &$\pm$5.0    &$\pm$8.9   &$\pm$5.0    &$\pm$8.2    &$\pm$3.6     &$\pm$5.1   &$\pm$11.3  &$\pm$5.2       &$\pm$2.4   &$\pm$2.9   &$\pm$11.1  &                         \\
                        & \multirow{2}{*}{LR}   & 84.12 & 73.78 & 85.33 & 66.55  & 66.66   & 69.04 & 57.20 & 69.21     & 42.25 & 53.43 & 64.30  & \multirow{2}{*}{66.53}   \\
                        &                       &$\pm$2.4   &$\pm$16.6  &$\pm$1.3   &$\pm$6.6    &$\pm$5.2     &$\pm$4.6   &$\pm$6.7   &$\pm$4.4       &$\pm$2.2   &$\pm$6.3   &$\pm$6.6   &                         \\
                        & \multirow{2}{*}{SVM}  & 83.96 & 77.10 & 85.27 & 64.36 & 68.32   & 71.20 & 55.55 & 71.65     & \textbf{43.00}    & 53.60  & 60.82 & \multirow{2}{*}{66.80}  \\
                        &                       &$\pm$2.3   &$\pm$12.9  &$\pm$2.0    &$\pm$8.3    &$\pm$4.3     &$\pm$4.9   &$\pm$5.6   &$\pm$3.9       &$\pm$2.7   &$\pm$6.0    &$\pm$12.4  &                         \\
                        & \multirow{2}{*}{SLP}   & \textbf{85.27} & 78.37 & 86.75 & \textbf{69.27} & 69.97   & 75.76 & \textbf{69.63} & 71.23     & 42.30  & 53.26 & \textbf{71.94} & \multirow{2}{*}{\textbf{70.34}}   \\
                        &                       &$\pm$2.1   &$\pm$8.2   &$\pm$1.8   &$\pm$7.2    &$\pm$4.8     &$\pm$4.5   &$\pm$0.3   &$\pm$7.9       &$\pm$3.1   &$\pm$2.3   &$\pm$2.7   &                         \\
                        & \multirow{2}{*}{GDA}  & 83.05 & 72.55 & 83.83 & 61.18 & 64.32   & 68.08 & 55.02 & 71.05     & 42.10  & 51.42 & 61.92 & \multirow{2}{*}{64.96}  \\
                        &                       &$\pm$3.1   &$\pm$8.5   &$\pm$1.7   &$\pm$17.2   &$\pm$8.2     &$\pm$5.3   &$\pm$5.6   &$\pm$4.8       &$\pm$2.1   &$\pm$3.1   &$\pm$10.8  &                         \\ 
    \hline
    \multicolumn{2}{c|}{\multirow{2}{*}{ICL}}   & 83.26 & \textbf{91.72} & \textbf{89.72} & 27.27  & \textbf{73.12}   & 71.60  & 34.28 & \textbf{73.02}     & 36.62 & \textbf{54.08} & 68.38 & \multirow{2}{*}{63.92}  \\
    \multicolumn{2}{c|}{}                       &$\pm$2.7   &$\pm$3.6   &$\pm$1.0    &$\pm$15.1   &$\pm$5.1     &$\pm$1.4   &$\pm$2.6   &$\pm$1.2       &$\pm$1.1   &$\pm$1.0    & $\pm$0.0     &                        \\
    \hline
    \end{tabular}

}
\caption{Experimental results on GPT-J in 8-shot per class settings. B, T, and D refers to a baseline, template, and demonstration individually. - means the case where ICL could not leverage full samples due to the length limitation. For each dataset, the \textbf{best method} is in bold. }

\label{tab:appendix_few-shot_8}
\end{table*}

\settowidth\rotheadsize{Minimal}
\begin{table*}[t]
\centering
\resizebox{2 \columnwidth}{!}{

    \begin{tabular}{c|c|cccccccccccc} 
    \hline
    \multicolumn{14}{c}{GPT-J 16-shot per class}                                                                                                                        \\ 
    \hline
    \multicolumn{2}{c}{Method}                  & AG    & SST-2 & RT    & Stance & Emotion & TREC  & CoLA  & Offensive & MNLI  & RTE   & MRPC  & AVG                     \\ 
    \hline
    \multirow{10}{*}{B} & \multirow{2}{*}{k-NN} & 69.6  & 52.75 & 66.94 & 63.27  & 40.37   & 70.92 & 49.72 & 61.7      & 35.75 & 53    & 58.87 & \multirow{2}{*}{55.33}  \\
                        &                       &$\pm$2.3   &$\pm$2.9   &$\pm$4.3   &$\pm$2.8    &$\pm$5.4     &$\pm$2.0    &$\pm$8.0    &$\pm$10.5      &$\pm$0.9   &$\pm$3.1   &$\pm$5.9   &                         \\
                        & \multirow{2}{*}{LR}   & 80.36 & 63.62 & 78.86 & 67.36  & 50.13   & 81.92 & 56.8  & 63.95     & 39.04 & 55.74 & 59.46 & \multirow{2}{*}{61.69}  \\
                        &                       &$\pm$2.0    &$\pm$2.5   &$\pm$4.1   &$\pm$3.9    &$\pm$3.3     &$\pm$3.4   &$\pm$5.9   &$\pm$8.5       &$\pm$1.7   &$\pm$2.4   &$\pm$5.6   &                         \\
                        & \multirow{2}{*}{SVM}  & 80.16 & 63.51 & 81.14 & 66.09  & 49.33   & 84.96 & 55.55 & 62.49     & 39.29 & 55.74 & 58.04 & \multirow{2}{*}{61.61}  \\
                        &                       &$\pm$2.1   &$\pm$5.0    &$\pm$3.7   &$\pm$3.2    &$\pm$4.1     &$\pm$1.8   &$\pm$6.2   &$\pm$9.7       &$\pm$2.1   &$\pm$2.5   &$\pm$5.2   &                         \\
                        & \multirow{2}{*}{SLP}   & 81.15 & 62.8  & 80.94 & 67.91  & 50.54   & 84.92 & 55.57 & 62.77     & 39.43 & \textbf{56.46} & 58.53 & \multirow{2}{*}{61.99}  \\
                        &                       &$\pm$2.0    &$\pm$4.3   &$\pm$3.8   &$\pm$5.1    &$\pm$4.9     &$\pm$2.1   &$\pm$5.9   &$\pm$7.9       &$\pm$1.9   &$\pm$3.2   &$\pm$4.7   &                         \\
                        & \multirow{2}{*}{GDA}  & 81.47 & 63.56 & 80.92 & 65.55  & 51.61   & \textbf{87.28} & 55.76 & 62.51     & 39.46 & 55.60  & 57.84 & \multirow{2}{*}{62.01}  \\
                        &                       &$\pm$1.9   &$\pm$5.0    &$\pm$3.6   &$\pm$3.3    &$\pm$4.1     &$\pm$1.8   &$\pm$6.3   &$\pm$9.6       &$\pm$1.8   &$\pm$2.6   &$\pm$4.9   &                         \\ 
    \hline
    \multirow{10}{*}{T} & \multirow{2}{*}{k-NN} & 74.25 & 76.28 & 74.54 & 59.73  & 57.21   & 68.44 & 46.67 & 58.6      & 38.07 & 51.99 & \textbf{67.25} & \multirow{2}{*}{59.88}  \\
                        &                       &$\pm$1.7   &$\pm$5.0    &$\pm$3.7   &$\pm$4.2    &$\pm$3.8     &$\pm$4.9   &$\pm$6.9   &$\pm$4.0        &$\pm$2.5   &$\pm$1.7   &$\pm$2.8   &                         \\
                        & \multirow{2}{*}{LR}   & 80.9  & 83.1  & 79.55 & \textbf{70.73}  & 67.22   & 83.2  & 54.78 & 68.95     & 42.73 & 56.61 & 64.85 & \multirow{2}{*}{67.17}  \\
                        &                       &$\pm$0.9   &$\pm$2.8   &$\pm$4.5   &$\pm$1.5    &$\pm$4.0      &$\pm$3.2   &$\pm$2.9   &$\pm$8.3       &$\pm$2.1   &$\pm$1.7   &$\pm$6.2   &                         \\
                        & \multirow{2}{*}{SVM}  & 82.3  & 83.97 & 80.86 & 67.73  & 67.01   & 85.4  & 55.36 & 67.98     & \textbf{44.15} & 55.96 & 65.78 & \multirow{2}{*}{67.42}  \\
                        &                       &$\pm$1.4   &$\pm$3.1   &$\pm$3.2   &$\pm$2.4    &$\pm$3.6     &$\pm$2.3   &$\pm$2.9   &$\pm$8.9       &$\pm$2.7   &$\pm$2.5   &$\pm$4.8   &                         \\
                        & \multirow{2}{*}{SLP}   & 83.11 & 84.54 & 81.29 & 69.73  & \textbf{69.02}   & 84.72 & \textbf{56.84} & \textbf{72.97}     & 44.13 & 56.25 & 66.23 & \multirow{2}{*}{\textbf{68.57}}  \\
                        &                       &$\pm$1.0    &$\pm$2.7   &$\pm$3.4   &$\pm$2.1    &$\pm$3.5     &$\pm$2.8   &$\pm$6.3   &$\pm$2.5       &$\pm$2.6   &$\pm$2.2   &$\pm$4.5   &                         \\
                        & \multirow{2}{*}{GDA}  & \textbf{83.63} & 83.83 & 80.69 & 67.55  & 67.04   & 86    & 55.46 & 67.84     & 44.48 & 56.17 & 66.13 & \multirow{2}{*}{67.52}  \\
                        &                       &$\pm$0.9   &$\pm$3.1   &$\pm$3.1   &$\pm$2.5    &$\pm$4.2     &$\pm$2.5   &$\pm$2.9   &$\pm$8.9       &$\pm$2.4   &$\pm$2.9   &$\pm$4.8   &                         \\ 
    \hline
    \multicolumn{2}{c|}{\multirow{2}{*}{ICL}}   & -     & \textbf{93.65} & \textbf{90.8}  & 23.73  & -       & 76.16 & 40.25 & 72.95     & -     & -     & -     & \multirow{2}{*}{-}  \\
    \multicolumn{2}{c|}{}                       & -     &$\pm$0.7   &$\pm$1.5   &$\pm$3.5    & -       &$\pm$3.0    &$\pm$8.0    &$\pm$0.5       & -     & -     & -     &                         \\ 
    \hline
    \end{tabular}
    
}
\caption{Experimental results on GPT-J in 16-shot per class settings. B, T refers to a baseline, template, and demonstration individually. - means the case where ICL could not leverage full samples due to the length limitation. For each dataset, the \textbf{best method} is in bold. }

\label{tab:appendix_few-shot_16}
\end{table*}
